# Supplementary material for: Analysis of the flow of granular materials through a screw conveyor
Source: arXiv:2111.13396 source file (2021-11-26)
Supplement: Supplementary file 1 [file appendix_a.tex]

\# 1\_pitch\_SI\_without\_grav\_6rpm\_full\\ 
log log\_1\_pitch\_SI\_without\_grav\_6rpm\_full.txt\\
\#\line(1,0){400}

\# Preliminaries\\
units si\\
atom\_style sphere\\
boundary f p s\\
newton off\\
communicate single vel yes\\
\#\line(1,0){400}

read\_data E:/f\_scratch/screw/p2d\_2/read\_data/fill\_data.txt\\                          
\#\line(1,0){400}

neighbor 0.0001 bin\\
neigh\_modify every 1 delay 0\\
\#\line(1,0){400}

\#  Material properties and interactions     \\                                    
fix m1 all property/global kn       peratomtypepair 1 12834.75  \\                  
fix m2 all property/global kt       peratomtypepair 1 3667.07\\
fix m3 all property/global gamman   peratomtypepair 1 0.04\\
fix m4 all property/global gammat   peratomtypepair 1 0.02\\
fix m5 all property/global coefficientFriction   peratomtypepair 1 0.5\\
\#\line(1,0){400}

\#  Contact physics\\
pair\_style gran model hooke/stiffness tangential history\\
pair\_coeff * *\\
\#\line(1,0){400}

\#  Integrator\\
fix integrate all nve/sphere\\
\#\line(1,0){400}

\#  Import mesh from cad:\\
fix cad1 all mesh/surface/stress file E:/f\_scratch/screw/p2d\_2/mesh/screw\_mid.stl type 1 scale 0.001 move 0.0 -0.076 0.0  curvature 1e-5 stress on\\
fix cad2 all mesh/surface/stress file E:/f\_scratch/screw/p2d\_2/mesh/shell.stl type 1 scale 0.001 curvature 1e-5 stress on\\
fix wall\_model all wall/gran model hooke/stiffness tangential history mesh n\_meshes 2 meshes cad1 cad2\\
\#\line(1,0){400}

\#  Timestep (t\_col/10)\\
timestep 0.0000022       \\                             
\#\line(1,0){400}

\#  Thermo settings\\
thermo\_style custom step atoms ke cpu\\
thermo 500\\
thermo\_modify lost ignore norm no flush yes\\
compute\_modify thermo\_temp dynamic yes\\
\#\line(1,0){400}

compute            peratom all stress/atom\\
\#\line(1,0){400}

\# get total force and torque of screw\\
variable time equal step*dt\\
variable fx equal f\_cad1[1]\\
variable fy equal f\_cad1[2]\\
variable fz equal f\_cad1[3]\\
variable Mx equal f\_cad1[4]\\
variable My equal f\_cad1[5]\\
variable Mz equal f\_cad1[6]\\
\#\line(1,0){400}

\# restart        1000000 restart/restart\_1\_pitch\_SI\_without\_grav\_6rpm\_full\_\\
\#\line(1,0){400}

\#  Make a dump of particles and the vtk file\\
dump  dmp all custom 5000 post/data*.vtk id type x y z ix iy iz vx vy vz fx fy fz omegax omegay omegaz radius c\_peratom[1] c\_peratom[2]\\ c\_peratom[3] c\_peratom[4] c\_peratom[5] c\_peratom[6]    \\

dump\_modify  dmp sort id\\

\# dump  dumpscrew\_int all mesh/vtk 5000 post/screw\_int*.vtk output interpolate stress stresscomponents cad1\\
dump  dumpscrew\_face all mesh/vtk 5000 post/screw\_face*.vtk output face id stress stresscomponents cad1\\

\# dump  dumpcase\_int all mesh/vtk 5000 post/case\_int*.vtk  output interpolate stress stresscomponents cad2\\
dump  dumpcase\_face all mesh/vtk 5000 post/case\_face*.vtk  output face stress stresscomponents cad2\\

fix forceslog all print 5000 "\$ {time},\$ {fx},\$ {fy},\$ {fz},\$ {Mx},\$ {My},\$ {Mz}" file post/forces.csv title "t,Fx,Fy,Fz,Mx,My,Mz" screen no \\
\#\line(1,0){400}

\#  Rotate the screw (specify the point through which the axis of rotation passes and the unit normal as per right hand rule)\\
fix movecad1 all move/mesh mesh cad1 rotate origin 0. 0. 0. axis 0. 1. 0. period -10.0  \#  6 RPM \\
\#\line(1,0){400}

run  20000000 upto\\
\#\line(1,0){400}
