# Supplementary material for: Analysis of the flow of granular materials through a screw conveyor
Source: arXiv:2111.13396 source file (2021-11-26)
Supplement: Supplementary file 2 [file appendix_c.tex]

\section{variation of quantities in the bulk}

\FloatBarrier
\subsection{Solid Fraction}
\begin{figure}[!htb]
	\centering
	\includegraphics[scale=0.42]{results/pitch_constant/solid_fraction.eps}
	\caption{Radial variation of solid fraction with scaled distance from the inner shaft for different gaps between the screw-shaft and the barrel}
\end{figure}

\FloatBarrier
\subsection{Pressure}
\begin{figure}[!htb]
	\centering
	\includegraphics[scale=0.42]{results/pitch_constant/pressure.eps}
	\caption{Radial variation of pressure with scaled distance from the inner shaft for different gaps between the screw-shaft and the barrel}
\end{figure}

\newpage
\subsection{Axial Velocity}
\begin{figure} [!htb]	
	\begin{subfigure}{\linewidth}
		\centering
		\includegraphics[scale=0.36]{results/pitch_constant/ax_vel_1.eps}
		\caption{}	
	\end{subfigure}\\[1ex]
	\begin{subfigure}{\linewidth}
		\centering
		\includegraphics[scale=0.36]{results/pitch_constant/ax_vel_2.eps}
		\caption{}
	\end{subfigure}
\caption{Radial variation of axial velocity with scaled distance from the inner shaft, for different gaps between the screw-shaft and the barrel. In (a) the velocities for the different cases are all scaled with the velocity at the tip of the screw flight corresponding to the smallest gap case, and in (b) the scaling for each case is with the corresponding axial velocity predicted by the theory for a frictionless screw.}
\end{figure}

\FloatBarrier
\subsection{Azimuthal Velocity}
\begin{figure} [!htb]	
	\begin{subfigure}{\linewidth}
		\centering
		\includegraphics[scale=0.36]{results/pitch_constant/az_vel_1.eps}
		\caption{}	
	\end{subfigure}\\[1ex]
	\begin{subfigure}{\linewidth}
		\centering
		\includegraphics[scale=0.36]{results/pitch_constant/az_vel_2.eps}
		\caption{}
	\end{subfigure}
\caption{Radial variation of azimuthal velocity with scaled distance from the inner shaft, for different gaps between the screw-shaft and the barrel. In (a) the velocities for the different cases are all scaled with the velocity at the tip of the screw flight corresponding to the smallest gap case, and in (b) the scaling for each case is with the corresponding azimuthal velocity adjacent to the barrel, predicted by the theory for a frictionless screw.}
\end{figure}

\FloatBarrier
\section{Stress variation on different surfaces of the screw} 

\FloatBarrier
\subsection{Barrel}

\begin{figure} [!htb]	
	\begin{subfigure}{\linewidth}
		\centering
		\includegraphics[scale=0.42]{results/pitch_constant/barrel_normal.eps}
		\caption{}	
	\end{subfigure}\\[1ex]
	\begin{subfigure}{\linewidth}
		\centering
		\includegraphics[scale=0.42]{results/pitch_constant/barrel_shear.eps}
		\caption{}
	\end{subfigure}
\caption{Variation of (a) normal stress and, (b) shear stress on the barrel with scaled distance from the trailing wing, for different gaps between the screw-shaft and the barrel. The inset shows the same thing on a semi-log graph.}
\end{figure}

\FloatBarrier
\subsection{Screw Root}

\begin{figure} [!htb]	
	\begin{subfigure}{\linewidth}
		\centering
		\includegraphics[scale=0.42]{results/pitch_constant/screw_root_normal.eps}
		\caption{}	
	\end{subfigure}\\[1ex]
	\begin{subfigure}{\linewidth}
		\centering
		\includegraphics[scale=0.42]{results/pitch_constant/screw_root_shear.eps}
		\caption{}
	\end{subfigure}
\caption{Variation of (a) normal stress and, (b) shear stress, on the screw-shaft with scaled distance from the trailing wing, for different gaps between the screw-shaft and the barrel. The inset shows the same thing on a semi-log graph.}
\end{figure}

\FloatBarrier
\subsection{Pushing/Trailing Wing}

\begin{figure} [!htb]	
	\begin{subfigure}{\linewidth}
		\centering
		\includegraphics[scale=0.265]{results/pitch_constant/push_normal.eps}
		\caption{}	
	\end{subfigure}\\[1ex]
	\begin{subfigure}{\linewidth}
		\centering
		\includegraphics[scale=0.265]{results/pitch_constant/push_tan_shear.eps}
		\caption{}
	\end{subfigure}
	\begin{subfigure}{\linewidth}
		\centering
		\includegraphics[scale=0.265]{results/pitch_constant/push_rad_shear.eps}
		\caption{}
	\end{subfigure}
	\caption{Radial variation of (a) normal stress, (b) tangential shear stress, and (c) radial shear stress, on the trailing wing, with scaled distance from the inner shaft for different gaps between the screw-shaft and the barrel.}
\end{figure}

\FloatBarrier
\subsection{Leading Wing}

\begin{figure} [!htb]	
	\begin{subfigure}{\linewidth}
		\centering
		\includegraphics[scale=0.265]{results/pitch_constant/lead_normal.eps}
		\caption{}	
	\end{subfigure}\\[1ex]
	\begin{subfigure}{\linewidth}
		\centering
		\includegraphics[scale=0.265]{results/pitch_constant/lead_tan_shear.eps}
		\caption{}
	\end{subfigure}
	\begin{subfigure}{\linewidth}
		\centering
		\includegraphics[scale=0.265]{results/pitch_constant/lead_rad_shear.eps}
		\caption{}
	\end{subfigure}
\caption{Radial variation of (a) normal stress, (b) tangential shear stress, and (c) radial shear stress, on the leading wing, with scaled distance from the inner shaft for different gaps between the screw-shaft and the barrel.}
\end{figure}
