# Supplementary material for: Analysis of the flow of granular materials through a screw conveyor
Source: arXiv:2111.13396 source file (2021-11-26)
Supplement: Supplementary file 3 [file appendix_b.tex]

The position and velocity of the particles are updated in the velocity-verlet algorithm \citep{swope1982computer} as follows.

\begin{enumerate}
	\item Calculate $\vec{v}(t+\frac{1}{2}\Delta t)=\vec{v}(t)+\frac{1}{2}\vec{a}(t)\Delta t^2$
	\item Calculate $\vec{x}(t+\Delta t)=\vec{x}(t)+\vec{v}(t+\frac{1}{2}\Delta t) \Delta t$
	\item Derive $\vec{a}(t+\Delta t)$ from the interaction potential using $\vec{x}(t+\Delta t)$
	\item Calculate $\vec{v}(t+\Delta t)=\vec{v}(t+\frac{1}{2}\Delta t)+\frac{1}{2}\vec{a}(t+\Delta t) \Delta t$
\end{enumerate}

\vspace{20 pt}
Eliminating the half-step velocity, this algorithm can be shorted to
\begin{enumerate}
	\item Calculate $\vec{x}(t+\Delta t)=\vec{x}(t)+\vec{v}(t)+\frac{1}{2}\vec{a}(t)\Delta t^2$
	\item Derive $\vec{a}(t+\Delta t)$ from the interaction potential using $\vec{x}(t+\Delta t)$
	\item Calculate $\vec{v}(t+\Delta t)=\vec{v}(t)+\frac{1}{2}(\vec{a}(t)+\vec{a}(t+\Delta t))\Delta t$
\end{enumerate}

The global error in the computation of position and velocity using the algorithm is $\mathcal{O}(\Delta t^2)$.
